# Supplementary material for: Enhancement in Thermally Generated Spin Voltage at Pd/NiFe$_2$O$_4$ Interfaces by the Growth on Lattice-Matched Substrates
Source: arXiv:2006.00777 ancillary file (2020-06-01)
Supplement: Supplementary file 1 [file Rastogi-SSE-NFO-Lattice-Matched-Substrates-Supplementary.pdf]

# Supplementary Information

## Enhancement in Thermally Generated Spin Voltage at Pd/$NiFe_2O_4$ Interfaces by the Growth on Lattice-Matched Substrate

A. Rastogi,[1,*] Z. Li,[1,2,*] A. V. Singh,[1] S. Regmi,[1,2] T. Peters,[3] P. Bougiatioti,[3] D. Carsten né Meier,[3] J. B. Mohammadi,[1,2] B. Khodadadi,[1,2] T. Mewes,[1,2] R. Mishra,[4] J. Gazquez,[5] A. Y. Borisevich,[6] Z. Galazka,[7] R. Uecker,[7] G. Reiss,[3] T. Kuschel,[3,†] and A. Gupta[1,‡]

[1]*Center for Materials for Information Technology,*
*The University of Alabama, Tuscaloosa, Alabama 35487, USA*

[2]*Department of Physics & Astronomy,*
*The University of Alabama, Tuscaloosa, Alabama 35487, USA*

[3]*Center for Spinelectronic Materials and Devices,*
*Department of Physics, Bielefeld University,*
*Universitätsstraße 25, 33615 Bielefeld, Germany*

[4]*Department of Mechanical Engineering and Materials Science,*
*and Institute of Materials Science and Engineering,*
*Washington University in St. Louis, St. Louis, Missouri 63130, USA*

[5]*Institut de Ciència de Materials de Barcelona,*
*Campus de la UAB, 08193, Bellaterra, Spain*

[6]*Materials Science and Technology Division,*
*Oak Ridge National Laboratory, TN 37831, USA*

[7]*Leibniz-Institut für Kristallzüchtung, Max-Born-Str. 2, 12489 Berlin, Germany*

(Dated: May 30, 2020)

## I. COMSOL Multiphysics® simulations

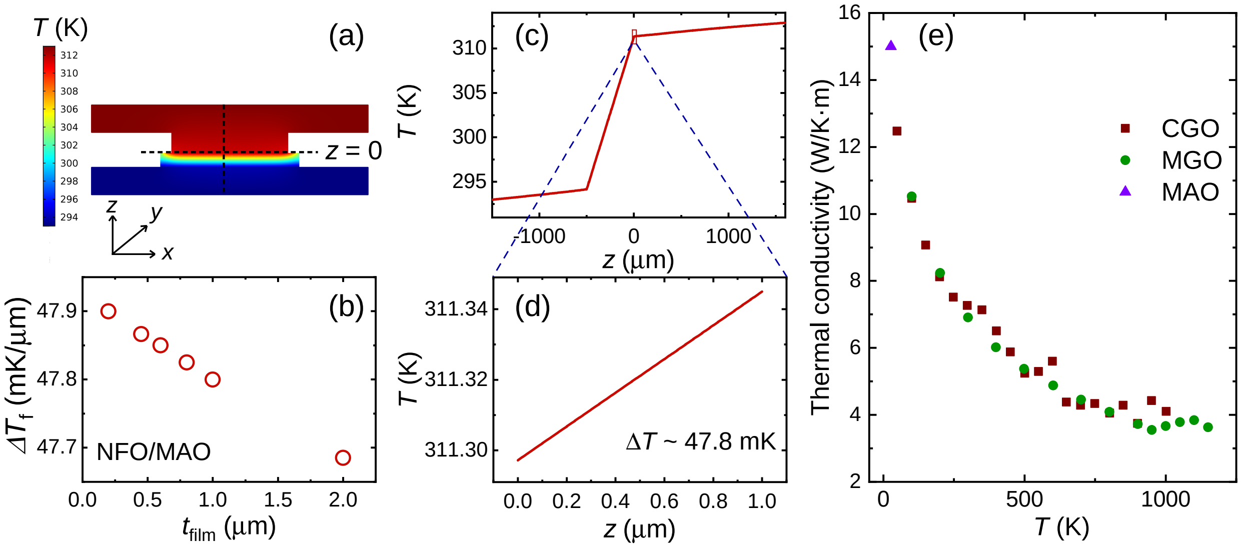


FIG. S1. (a), (b), (c), and (d) are the results of COMSOL simulation. In panel (a), $z = 0$ indicate the substrate of the top surface, and the film thickness is 1 μm. (b) Simulated temperature gradient across the different thickness NFO films on MGO substrates. (c) Temperature profile of the stack along z-direction (perpendicular to $z = 0$), while (d) shows the temperature variation across only the film. (e) Thermal conductivity data for the three single crystal substrates used for our experiments. The data for MGO is taken from Ref. [1].

| Material | Density (kg/m$^3$) | Thermal conductivity (W/(K· m)) | Heat capacity (J/(kg· K)) |
|---|---|---|---|
| Cu [1] | 8960 | 401 | 384 |
| SiC [1] | 3216 | 490 | 690 |
| Pd [1] | 12020 | 71.8 | 244 |
| $NiFe_2O_4$ [2] | 5227 | 11.1 | 600 |
| $MgAl_2O_4$ [1] | 3579 | 15.5 | 805 |
| $MgGa_2O_4$ [3] | 5296 | 12 | 600 |

TABLE S1. Material parameters such as density, thermal conductivity, and heat capacity used for COMSOL Multiphysics® simulation.

For COMSOL Multiphysics® simulations, we used the steady-state solution of heat transfer in a solid to estimate the temperature profile across the stack. We adopted the swept meshing

method with minimum element size of 50 nm. In the region of interest, i.e. (film + Pd), a mesh distribution was applied to further reduce the size. Initially, the system temperature was chosen as 293 K with the hot (top) and cold (bottom) end at 313 K and 293 K, respectively. Fig. S1(a) shows the cross-sectional view of temperature distribution across the stack.

In Fig. S1(b) we present the simulated temperature gradient ($\Delta T_{\mathrm{f}}$) for different NFO film thicknesses on MGO substrate. The result shows that $\Delta T_{\mathrm{f}}$ is in the range of tens of milliKelvin when a temperature difference $\Delta T \approx 20$ K is applied across the Cu blocks. Thus, nearly the same temperature gradient is generated irrespective of the film thickness when the same $\Delta T$ is applied across the Cu blocks. The variation of temperature across the stack is shown in Fig. S1(c) and the temperature profile across a 1 μm thick NFO film is displayed in Fig. S1(d). Furthermore, we find that the temperature difference across the film scales with the temperature difference across the Cu-blocks. The material parameters used for the COMSOL simulation are listed in Table S1. Based on similar thermal conductivity values shown in Fig. S1(e), for simulation the thermal conductivity of CGO, MGO, and MAO (Table S1), we find that the temperature gradient across the films are in very similar range.

## II. Spin Seebeck effect measurements of NFO films on different substrates

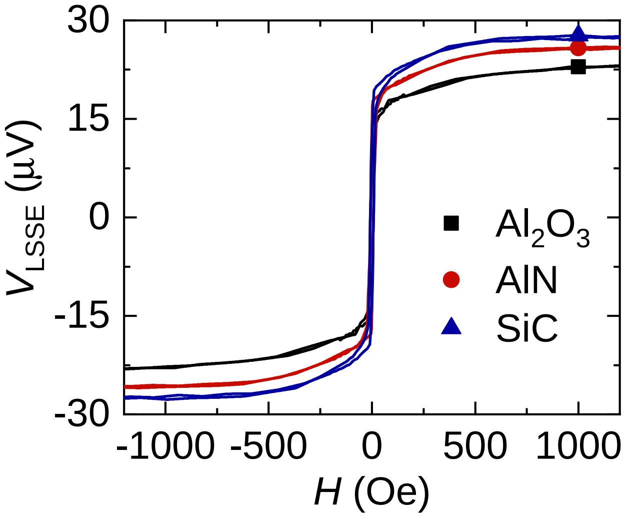


FIG. S2. The variation of $V_{ISHE}$ signal for 1 μm thick NFO film grown on CGO substrate measured at $\theta$ = 90° with different electrically insulating spacer substrates.

Figure S2 shows the result of SSE voltage signal comparison using three different insulating spacers ($Al_2O_3$, AlN, SiC), which indicates that SiC has the best thermal conductivity.

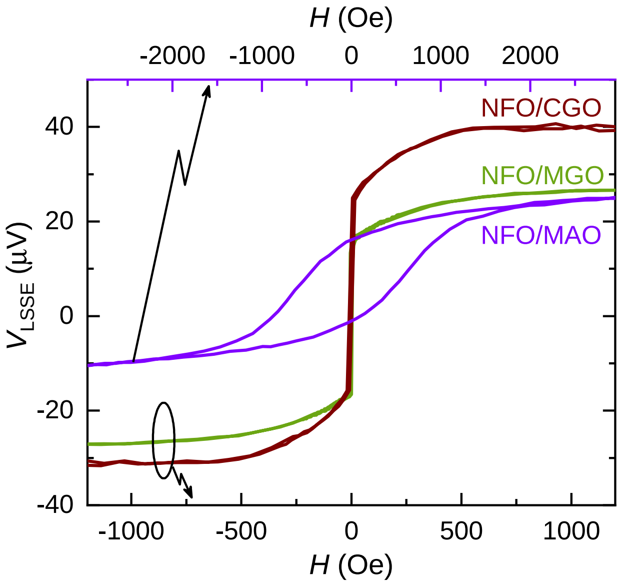


FIG. S3. Magnetic field dependence (± 1200 Oe for NFO/CGO and NFO/MGO, ± 3000 Oe for NFO/MAO) of the $V_{\mathrm{ISHE}}$ signal plotted for the 330 nm thick films deposited on different substrates.

Figure S3 presents full magnetic field sweep scan data for 330 nm NFO films on the three substrates without any background subtraction.

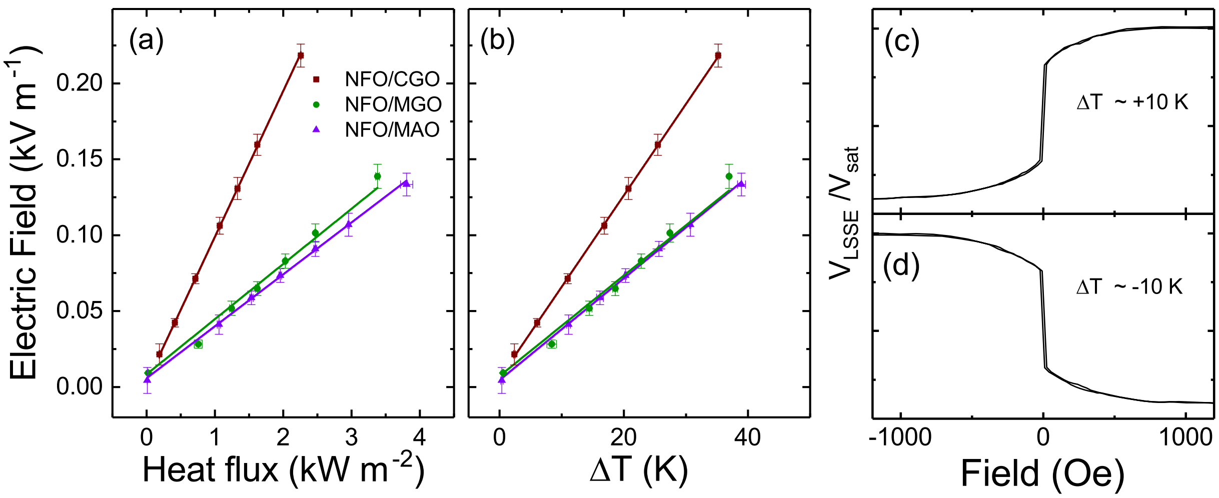


FIG. S4. The variation of saturation ISHE electric field with (a) heat flux and (b) temperature gradient method for 60 nm thick NFO films grown on CGO, MGO and MAO substrates, respectively. The points are the measured values, while the solid lines are the linear fits. Plots (c) and (d) show the normalized electric field with change in the direction of temperature gradient $\Delta T$ from $\sim$ +10 K to $\sim$ -10 K, respectively.

Figures S4(a) and S4(b) show the saturation electric field generated in the Pd layer depending on the heat flux ($\Phi_q$) and the temperature difference ($\Delta T$). As expected, we observe a linear relationship. When the direction of $\Delta T$ is reversed the sign of $E_{\rm ISHE}$ also reverses (Fig. S4(c)). This is a characteristic behavior of $E_{\rm ISHE}$ induced by LSSE.

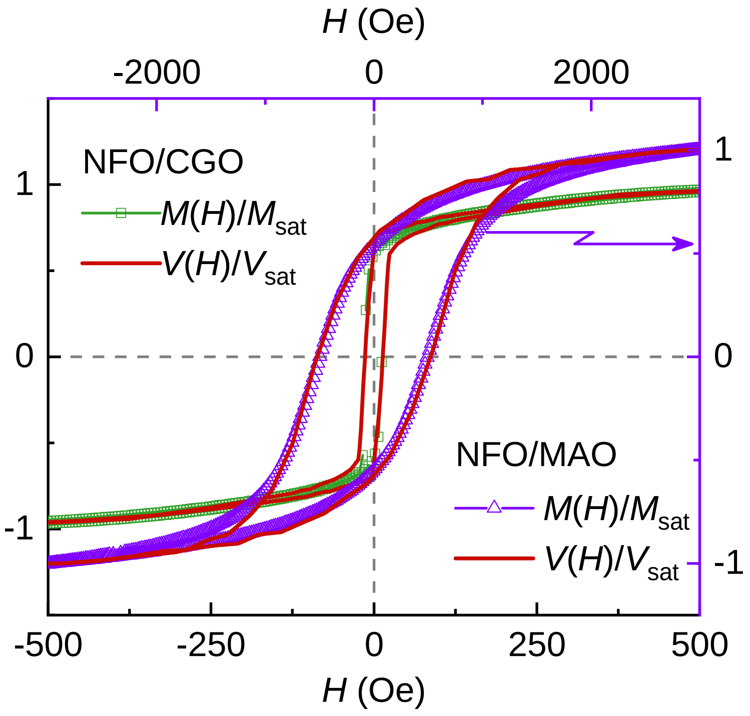


FIG. S5. A comparison between the normalized values of M(H) and V(H) measured by VSM and $V_{LSSE}$, respectively, for NFO films (1 μm) grown on CGO and MAO substrates.

Figure S5 displays normalized magnetization curves and their resemblance with the normalized voltage signals ($\theta \approx 90^\circ$). The data shown here are for two samples NFO/CGO (lower scale) and NFO/MAO (top scale), respectively.

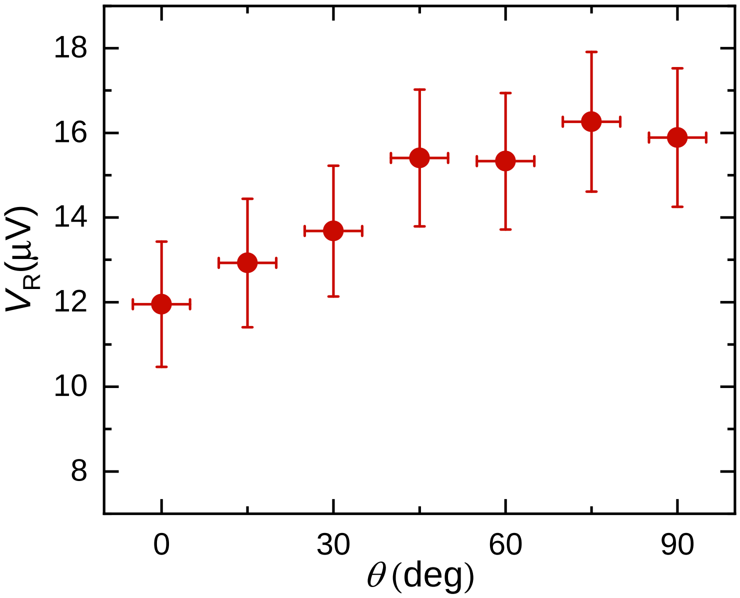


FIG. S6. Variation of the remanent voltage $V_R$ with angle ($\theta$) for 330 nm thick NFO film on MGO substrate.

In Figure 4(e) of the main text, we observe a non-zero voltage signal at smaller fields for 0°, and the voltage signal is comparable to $\theta = 90°$. We studied the angular dependency of the $V_{ISHE}$ signal with magnetic field by varying $\theta$ in the range 0° to 90° and the remanent voltage ($V_R$) with $\theta$ is plotted Fig. S6.

## III. Spin Seebeck measurements of NFO films grown on (011)-oriented MGO substrates

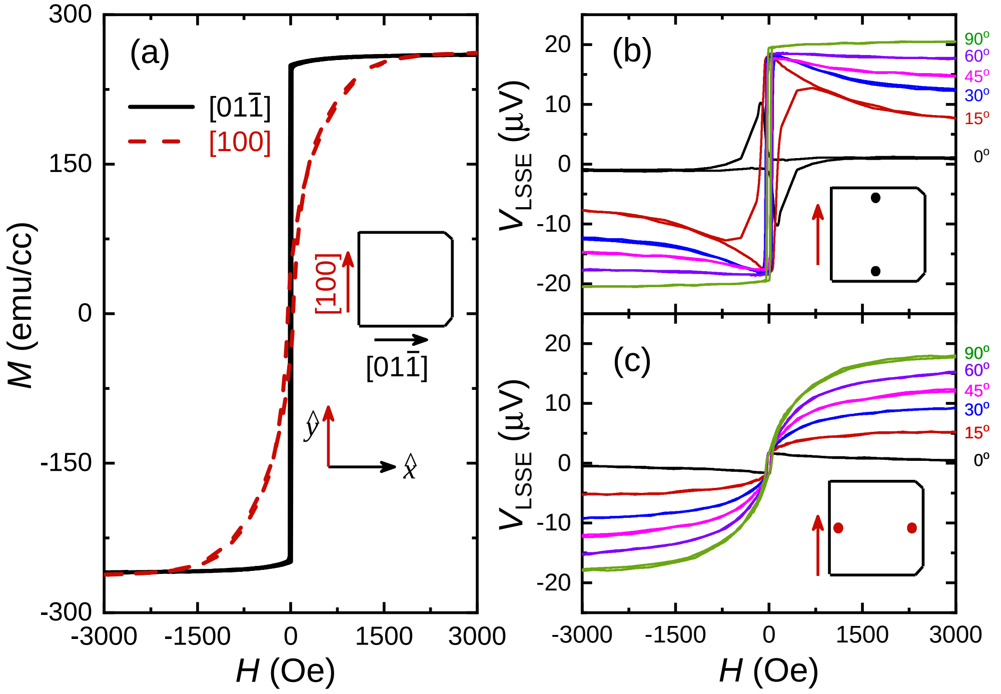


FIG. S7. (a) Variation of magnetization with magnetic field for a 330 nm thick NFO/MGO (011) film. The magnetization is measured with the external in-plane magnetic field applied in the direction of the magnetic easy axis [01$\bar{1}$] (black line) and the magnetic hard axis [100] (red line), respectively. LSSE measurements at various angles for Pd/NFO/MGO with voltage being measured (b) along the [100] direction and (c) along the [01$\bar{1}$] direction, respectively.

Magnetization measurements have been performed on a 330 nm thick $NiFe_2O_4$ film grown on (011)-oriented $MgGa_2O_4$ substrate to examine the in-plane magnetic anisotropy. As shown in Fig. S7(a), we observe a sharp switching of the magnetization when the external magnetic field is applied along the magnetic easy axis [1$\bar{1}$0], with a squareness of approximately one. With the external magnetic field applied along the magnetic hard axis ([001]), we obtain switching behavior associated with a magnetic hard axis with an anisotropy field of about 2000 Oe, and squareness far less than one. We measured the $V_{ISHE}$ signal in two configurations. In the first configuration the $V_{ISHE}$ signal is measured along the magnetic hard axis of the $NiFe_2O_4$ film, i.e., along the $\hat{y}$-direction (Fig. S7(b)), and in the other case the $V_{ISHE}$ signal is measured along the magnetic easy axis, i.e., along the $\hat{x}$-direction (Fig. S7(c)).

In the first configuration, we measure the voltage signal along the magnetic hard axis, i.e.,

along the [100] direction. When the magnetic field is applied along the magnetic easy axis, i.e. along the [01$\bar{1}$] direction, the magnetization of the $NiFe_2O_4$ film also aligns along the same direction and when the magnetic field direction changes polarity the magnetization switches into the opposite direction. This results in a sharp switching in the $V_{ISHE}$ signal (90° in Fig. S7(b)) and it is comparable to the corresponding magnetization measurement when the magnetic field is applied in the [01$\bar{1}$] direction (Fig. S7(a)). In the next step, we changed the angle $\theta$ of the external magnetic field with respect to the voltage measurement direction, i.e., from the $\hat{y}$-direction in the range from 0° to 90°. In saturation, the magnetization of the $NiFe_2O_4$ is aligned along the direction of the external magnetic field for all $\theta$ angles. The direction of the voltage measurement is only sensitive for the detection of the spin current that is spin polarized along the $\hat{x}$-direction. The voltage generation due to ISHE arises from the projection of the magnetization in the $\hat{x}$-direction. Upon lowering the angle between the external magnetic field and the $\hat{y}$-direction, the saturation voltage decreases in correspondence with cross product in the ISHE equation. When the magnetic field decreases, the magnetization rotates coherently into the magnetic easy axis. The projection of the magnetization in the $\hat{x}$-direction increases which also increases the measured voltage by the ISHE. At zero magnetic field the magnetization rotates completely into the magnetic easy axis. This occurs for all angles $\theta$ up to 15°, which results in nearly the same voltage signal. Subsequently, when the magnetic field polarity is changed the magnetization switches into the opposite direction along the magnetic easy axis. Upon increasing the magnetic field in the negative direction the measured voltage decreases in corresponding to a coherent rotation of the magnetization into the magnetic field direction. For lower angles $\theta$, the magnetization switching deviates more and more from the sharp switching behavior observed for larger angles. For 15° and 0°, i.e., near the magnetic hard axis, we observe a behavior corresponding to presence of multiple domains. The domains rotate clockwise or counter-clockwise into the next magnetic easy axis. This leads to an intermediate voltage for 0° around zero magnetic field which is smaller than the observed value when all domains rotate into the same direction.

In the second configuration, we changed the position of the voltage contacts and measured the $V_{ISHE}$ signal along the magnetic easy axis. When the external magnetic field is applied along the magnetic hard axis to complete the typical LSSE configuration, i.e., $\theta = 90°$, we observe an LSSE voltage curve similar to the magnetization curve along the magnetic hard axis ([100] direction in Fig. S7(a)). The LSSE signal saturates at the highest applied external magnetic field. When the external magnetic field is reduced the LSSE voltage does not show a sharp switching, but favors

the curved shape of the magnetization measurement in the [100] direction with low remanence. While the projection of the magnetization into the $\hat{y}$-direction decreases monotonically, the LSSE voltage also decreases. After changing the polarity of the magnetic field, the magnetization switches by 180° into the magnetic easy axis, which is along the voltage contacts. This results in a nearly zero voltage signal. When the magnetic field increases again in the negative direction, the magnetization rotates back into the magnetic field direction. The projection into the $\hat{y}$-direction as well as the absolute value of the $V_{\mathrm{ISHE}}$ increases, because the electric field along the voltage contacts increases due to the ISHE. The saturation voltage follows, again, the cross product of the ISHE and can be compared to the saturated voltage in Fig. S7(b). The slight differences can be explained by misalignments of the voltage contacts and the direction of the magnetic field. For angles $\theta$ larger than 0° (Fig. S7(c)), the saturation voltage increases (decreases) for positive (negative) magnetic fields similar to the configuration in Fig. S7(b). When the magnetic field is reduced the curves for $\theta$ between 15° and 60° can be explained in the same manner as for $\theta = 90°$. For $\theta = 0°$ the saturation voltage is nearly zero as expected, but around zero magnetic field the measured voltage increases (decreases) when the external magnetic field is decreased (increased). Here, we expect an accurate alignment with the voltage contacts, but a misalignment of the voltage contacts with respect to the magnetic easy axis. This results in a slight voltage contribution at zero field when the magnetization rotates into the magnetic easy axis. The LSSE measurements provide an attractive alternative to investigate in-plane magnetic anisotropies by varying the direction of the voltage contacts and the angle of the external magnetic field. The alignment accuracy between the voltage contacts, and the external magnetic field with respect to the magnetic easy axis can in principle be controlled very precisely.

## IV. Results of ferromagnetic resonance (FMR) measurements

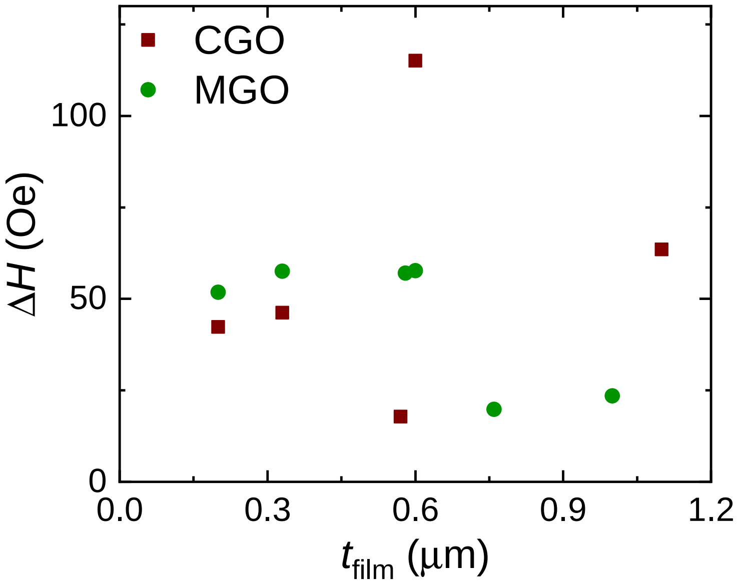


FIG. S8. Variation of FMR line-width as a function of NFO film thickness for two different substrates.

In Figure S8, we show the thickness variation of FMR line-width ($\Delta H$) of NFO films deposited on MGO and CGO substrate. The films deposited on CGO substrate show scattered data points. For film thicknesses $\leq$ 330 nm $\Delta H$ is larger than that of the films deposited on MGO substrate. In contrast, for film thicknesses $\geq$ 600 nm $\Delta H$ is larger for films on CGO. The data correlates well with the observation of SSE measurements using heat flux method (Fig. 5(c)) in the main text.

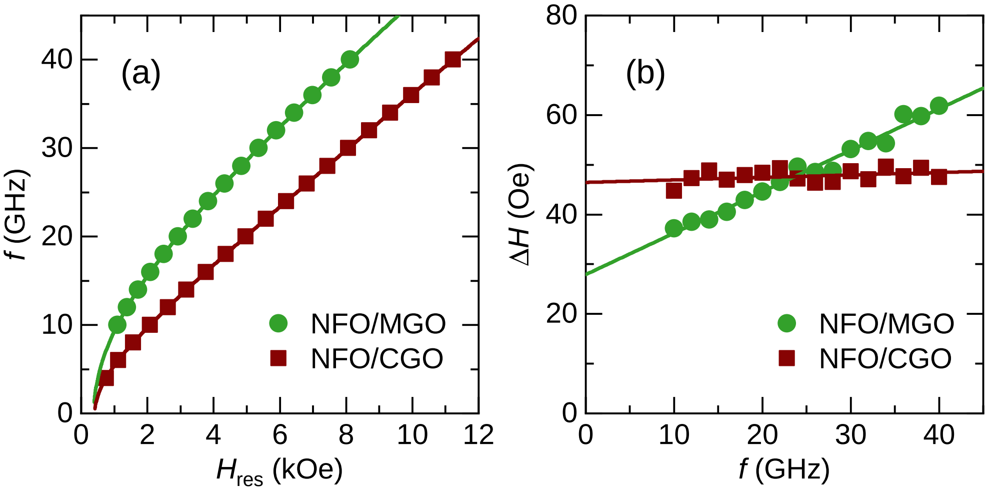


FIG. S9. Broadband FMR measurement results of 330 nm thick NFO films without Pd top layer deposited on CGO and MGO substrates. (a) Microwave frequency vs. resonance field data (symbols) are fitted to Kittel's equation (solid lines). (b) The dependence of FMR line width signal with resonance frequency (solid data points) and solid lines are fits to calculate the effective Gilbert damping and inhomogeneous linewidth broadening.

In Figure S9, we show FMR measurement results of 330 nm thick NFO films without Pd top layer deposited on CGO and MGO substrates. To estimate the effective magnetization ($M_{\mathrm{eff}}$) and gyromagnetic ratio ($\gamma'$), we fit the frequency ($f$) versus resonance field ($\mathrm{H_{res}}$) data (Fig. S9(a)) to the Kittel equation in the in-plane configuration using equation

$$f = \gamma' \sqrt{(H_{\mathrm{res}} + H_4) \cdot (H_{\mathrm{res}} + H_4 + 4\pi M_{\mathrm{eff}})}, \tag{1}$$

where $H_4$ is the four-fold in-plane anisotropy.

The FMR linewidth ($\Delta H$) vs. frequency ($f$) data (Fig. S9(b)) is then used to calculate the effective Gilbert damping parameter ($\alpha_{\mathrm{eff}}$) and inhomogeneous linewidth broadening ($\Delta H_0$)using equation,

$$\Delta H = \Delta H_0 + \frac{2\alpha_{\mathrm{eff}}}{\sqrt{3}\gamma'} f. \tag{2}$$

The estimated value of the $\alpha_{\mathrm{eff}}$ of the NFO/MGO and NFO/CGO thin films without Pd top layer are determined to be $(22 \pm 0.9) \times 10^{-4}$ and $(1.3 \pm 0.9) \times 10^{-4}$, respectively.

* These authors contributed equally to this work.

† E-mail: tkuschel@physik.uni-bielefeld.de

‡ E-mail: agupta@mint.ua.edu

[1] Comsol multiphysics material library, https://www.comsol.com/material-library.

[2] A. T. Nelson, J. T. White, D. A. Andersson, J. A. Aguiar, K. J. McClellan, D. D. Byler, M. P. Short, and C. R. Stanek, J. Am. Ceram. Soc. **97**, 1559 (2014).

[3] K. R. Wilkerson, J. D. Smith, T. P. Sander, and J. G. Hemrick, J. Am. Ceram. Soc. **96**, 859 (2013).
